# Supplementary material for: An Informatics Framework for the Design of Sustainable, Chemically Recyclable, Synthetically-Accessible and Durable Polymers
Source: arXiv:2409.15354 ancillary file (2024-09-13)
Supplement: Supplementary file 1 [file supplementary.pdf]

# Supplementary: An Informatics Framework for the Design of Sustainable, Chemically Recyclable, Synthetically-Accessible and Durable Polymers

Joseph Kern,† Yongliang Su,‡ Will Gutekunst,‡ and Rampi Ramprasad*,†

†*School of Materials Science and Engineering, College of Engineering, Georgia Institute of Technology, 771 Ferst Dr. N.W., Atlanta, GA 30318, U.S.A.*

‡*School of Chemistry & Biochemistry, College of Sciences, Georgia Institute of Technology, 901 Atlantic Drive NW, Atlanta, GA 30318, U.S.A.*

E-mail: rampi.ramprasad@mse.gatech.edu

## Design Analysis

Figure S1 illustrates the correlation between rings within a known polymer (whether ROP or not) and key properties such as glass transition temperature ($T_g$), melting temperature ($T_m$), tensile strength at break ($\sigma_b$), and Young's modulus (E) based on our experimental dataset. Our analysis reveals a consistent and statistically significant rightward shift in the histograms associated with each property when the polymer incorporates a ring (whether aromatic or aliphatic). Notably, for $T_g$, E, and $\sigma_b$, this shift is prominently observed when the ring is situated within the polymer backbone. However, such a dependence on backbone placement is not uniformly observed for $T_m$. While the rightward trend appears notably pronounced for both classes of properties, caution is warranted regarding mechanical properties due to the relatively small dataset size of polymers devoid of rings.

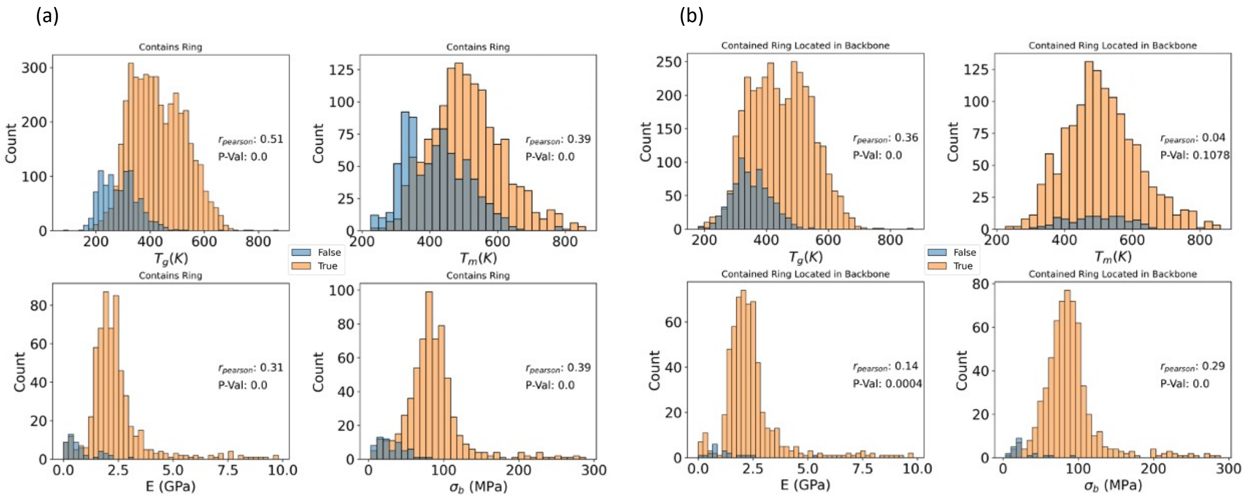


Figure S1: Histograms showcasing the distribution of measured $T_g$, $T_m$, $\sigma_b$ and E according to whether the polymer contains a ring (a), and if the contained ring is in the backbone of the polymer (b). Pearson correlations are presented as well as the P-value rounded to the fourth decimal.

In Figure S2 (a) and (b), we present the impact of amines/(thio)amides and (thio)imides on the known polymer properties respectively. For all properties, (thio)imides cause a statistically significant (P-value $< 0.05$) shift rightward in properties. Amines/(thio)amides seem to influence thermal properties, but not mechanical. In (c) we evaluate the impact of H-bond acceptor atoms (like those in primary/secondary amines and amides) on the properties and see a trend that increasing the number of H-Bond acceptor atoms increases the properties.

Interestingly, a positive correlation emerges between thermal and mechanical properties. As depicted in Figure S3, the plot of measured $T_g$ versus $\sigma_b$ reveals a robust Pearson correlation coefficient of 0.64 between these properties. Additional correlations between other polymer properties can be found in[1]

# Thiocane Synthesis

The monomer TC-Ph and TC-Fr were prepared according to the procedures reported in the literature with some modifications.

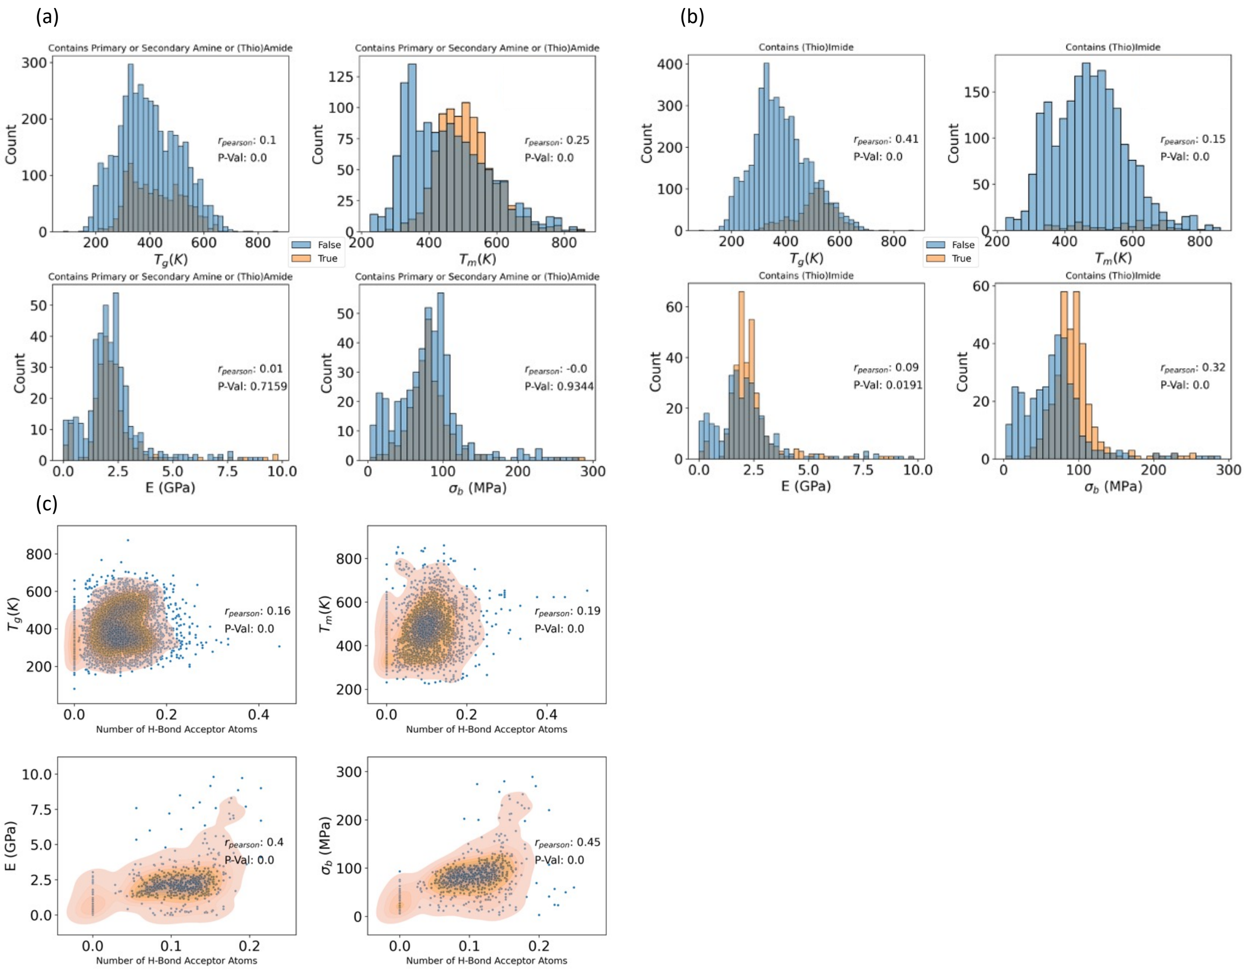


Figure S2: Histograms showcasing the distribution of measured $T_g$, $T_m$, $\sigma_b$ and E according to whether the polymer contains an amine or (thio)amide (either =O or =S) (a), or contains a (thio)imide (any combination of =O and =S) (b). (c) Pair plot illustrating the effect of H-bond acceptor atom count normalized by polymer atom count on various properties. A two-dimensional kernel density estimate (KDE) plot is overlaid to display to density of points. Pearson correlations are presented as well as the P-value rounded to the fourth decimal.

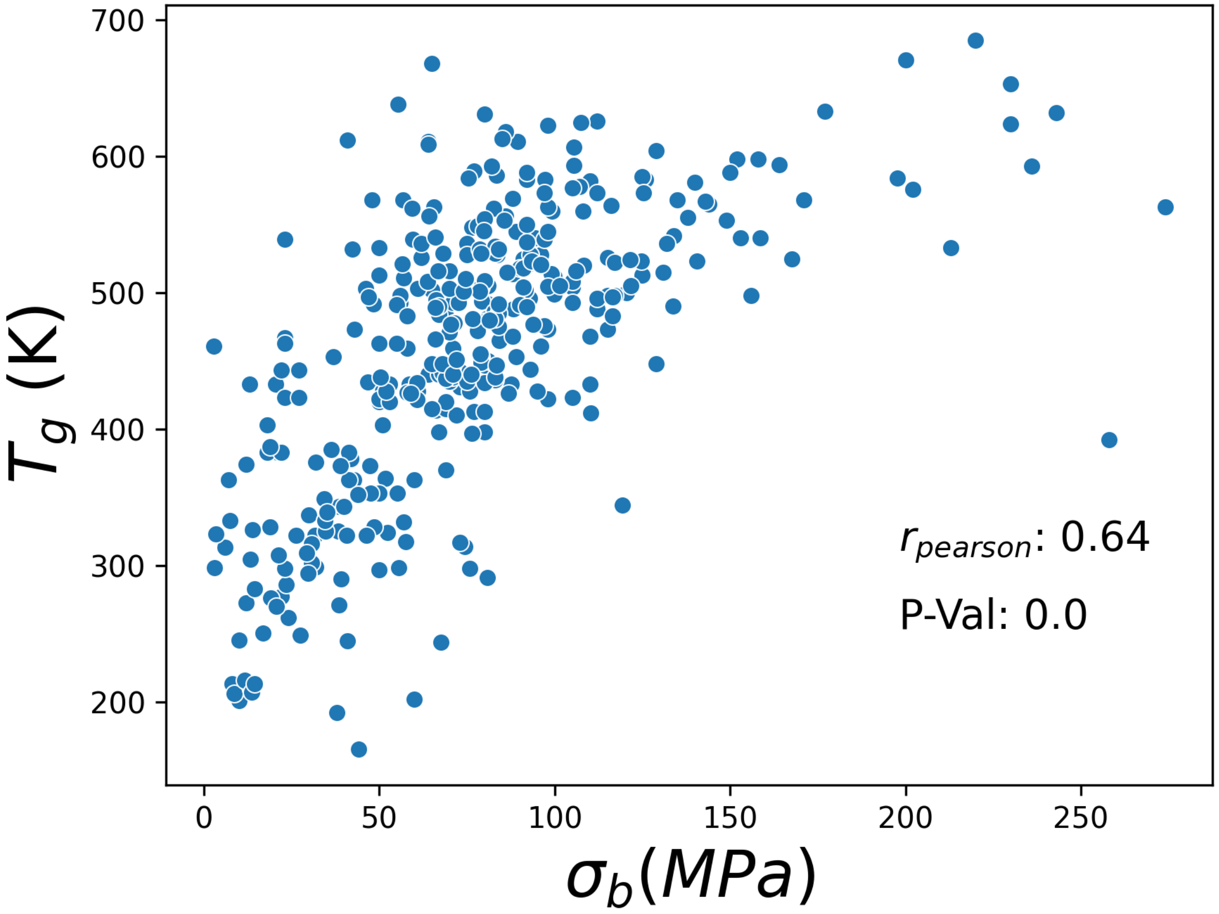


Figure S3: Pairwise plot of experimental glass transition temperature vs tensile strength at break. Pearson correlations are presented as well as the P-value rounded to the fourth decimal.

## Representative Procedure for Friedel-Crafts Acylation of Alkynes

To a stirred suspension of aluminum chloride (10.47 g, 78.5 mmol) in dry dichloromethane (40 ml) at 0 ℃, was added a mixture of phenylacetylene (7.29 g, 7.84 mL, 71.4 mmol) and 5-chloropentanoyl chloride (11.06 g, 9.17 mL, 71.4 mmol) dropwise over 10 min. The cooling bath was removed, and the reaction mixture was warmed up to ambient temperature over one hour. The mixture was poured into a mixture of brine and ice. The mixture was stirred for two hours at ambient temperature and extracted using dichloromethane (60 mL×3). The combined organic layers were washed with brine and dried over magnesium sulfate and concentrated in vacuo. The residue was purified by column chromatography on silica gel (eluent: hexanes/diethyl ether = 10:1) to give the alkene product (pale yellow solid, 70% yield, 12.85 g). The spectral data were in accordance with those reported in the literature.[2]

## Modified Procedure for Cyclization with KSAc

To a stirred solution of (Z)-1,7-dichloro-1-phenylhept-1-en-3-one (13.5 g, 52.5 mmol) in DMF (260 mL, 0.2 M) was added potassium thioacetate (KSAc, 53 mmol, 6.05 g) at ambient temperature. The reaction was complete in 5 h as evidenced by thin layer chromatography. The reaction mixture was diluted with H2O (200 mL), then extracted with ethyl acetate (150 mL×3). The combined organic layers were washed with H2O (150 mL×3), dried over magnesium sulfate and concentrated in vacuo. The crude product was used in next step without purification. To a stirred solution of above obtained crude product in MeOH (500 mL, 0.01 M) was added potassium carbonate (K2CO3, 57.75 mmol, 7.98 g) at 0 ℃. The reaction was allowed to warm up to ambient temperature slowly. After stirred for another 5 h, the reaction mixture was quenched with HCl (30 mL, 2 M), then extracted with ethyl acetate (150 mL×3). The combined organic layers were washed with brine, dried over magnesium sulfate and concentrated in vacuo. The residue was purified by column chromatography on silica gel (eluent: hexanes/ ethyl acetate = 10:1) to give the thiocane monomer (pale yellow solid, 49% yield in two steps, 5.6 g). The spectral data were in accordance with those

reported in the literature.[2]

## General Polymerization Procedure for the Synthesis of Polythiocanes

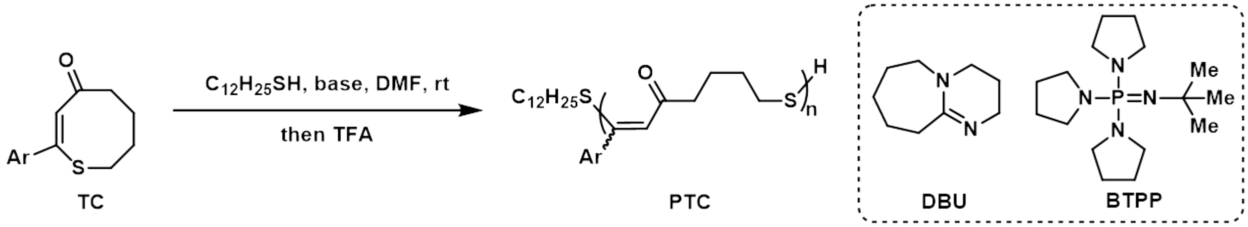


Figure S4: Polymerization procedure for the synthesis of polythiocanes.

Preparation of stock solution: The desired amounts of 1-dodencanethiol and base were added into an oven-dried 2 mL vial under N2. Dry, degassed DMF was then added to make a stock solution.

To an oven-dried microwave vial equipped with a magnetic stir bar was added the thiocane monomer TC (0.2 mmol). Following the evacuation and triple backfilling with N2, the vial was charged with dry, degassed DMF, along with the initiator stock solution. After stirring for the indicated time, the reaction was quenched by three drops of trifluoracetic acid. An aliquot of the reaction mixture was taken for 1H NMR to determine the conversion of the monomer. Another aliquot of the reaction mixture was taken for SEC analysis. The resulting polymer was precipitated from cold MeOH. The purified polymer was then characterized using SEC, 1H-NMR, 13C-NMR, TGA and DSC.

# VFS and the Database Schema

We use a relational structured query language (SQL) PostgreSQL database to store results for our virtual forward synthesis (VFS) technique. The database, shown in Figure S5, houses the molecules and reactions used for virtual forward synthesis, as well as the polymers and

their predicted properties that result from it. The first step in the VFS process is creating a catalog of commercially available and known molecules.

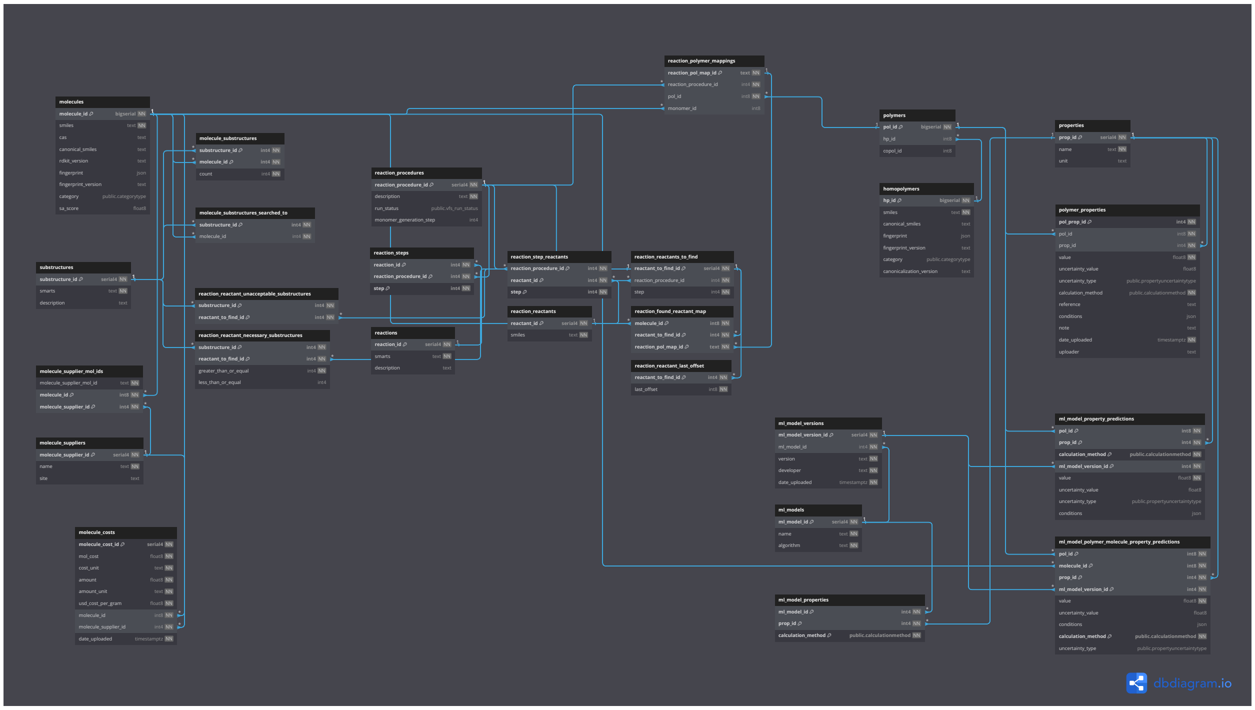


Figure S5: VFS database schema

All tables specific to molecules are located on the left hand side of Figure S5. During the cataloging, each molecule is assigned a unique identifier and stored alongside its simplified molecular-input line-entry system (SMILES) notation, canonical SMILES representations, synthetic accessibility score (SAScore), categorization (whether real or hypothetical), and fingerprints. Furthermore, comprehensive details such as which sources reference the known or commercially available molecules and the distinct molecule IDs assigned by suppliers are maintained in a separate table that links to the molecules table via a foreign key. Additionally, if a molecule was discovered through our web scraping efforts (as detailed in Section "Webscraper"), we keep track of its price data[1]. We implement B-Tree indices on the molecules based on their canonical SMILES and categorization to significantly enhance

[1]While we maintain a table for suppliers, it primarily serves to record unique IDs from various databases such as eMolecules, ChemBL, Zinc15, or VWR, which are often intermediary references for the true suppliers. Therefore, the term "supplier" may not entirely encapsulate the function of this table.

query efficiency of molecules from O(n) to O(log(n)). This approach guarantees that each molecule is stored only once in the table. It is particularly crucial during the VFS process, where we aim to query only known molecules, thereby streamlining the entire procedure.

The VFS process occurs in three steps. First, a detailed reaction procedure is crafted to outline the sequential reaction steps, specify necessary and unacceptable substructures within each variable reactant, and include additional reactants essential for the process. Following this, molecules are searched for all of the necessary and unacceptable substructures. Subsequently, each molecule containing all of the necessary substructures and none of the unacceptable ones progresses through the predefined reaction steps, yielding polymers as outputs, which are cataloged and securely stored within the database. An illustrative example of this process is shown in Figure S6.

The VFS reaction procedure unfolds through a series of reaction steps. Each step is delineated by its reaction SMARTS, which outlines the desired chemical transformation. These reaction SMARTS are archived in the reactions table, while the step itself is recorded in the reaction steps table, linking to the reactions table via the reaction ID, as shown in Figure S5. Within each reaction step, reactants can be extracted from the molecule database based on user-defined necessary and unacceptable substructures. These necessary substructures are typically contingent upon the specific reaction being executed. For instance, in the context of Figure S6, the essential substructure for the variable reactant in the initial reaction step is identified as an ester within a ring.

Moreover, each step can incorporate additional reactants provided by the user, such as the sulfur atom in step 1 of Figure S6 and the germanium atom in step 2. While these may be crucial for the progression of the reaction, they need not necessarily be variable. Additionally, while the real chemical reaction typically requires the sulfur to be donated from some molecule, in synthetic reactions we can simply swap the elements. The initial output from each reaction step serves as input for the subsequent reaction step, ensuring a seamless continuation of the process. Furthermore, within the reaction procedure, it is

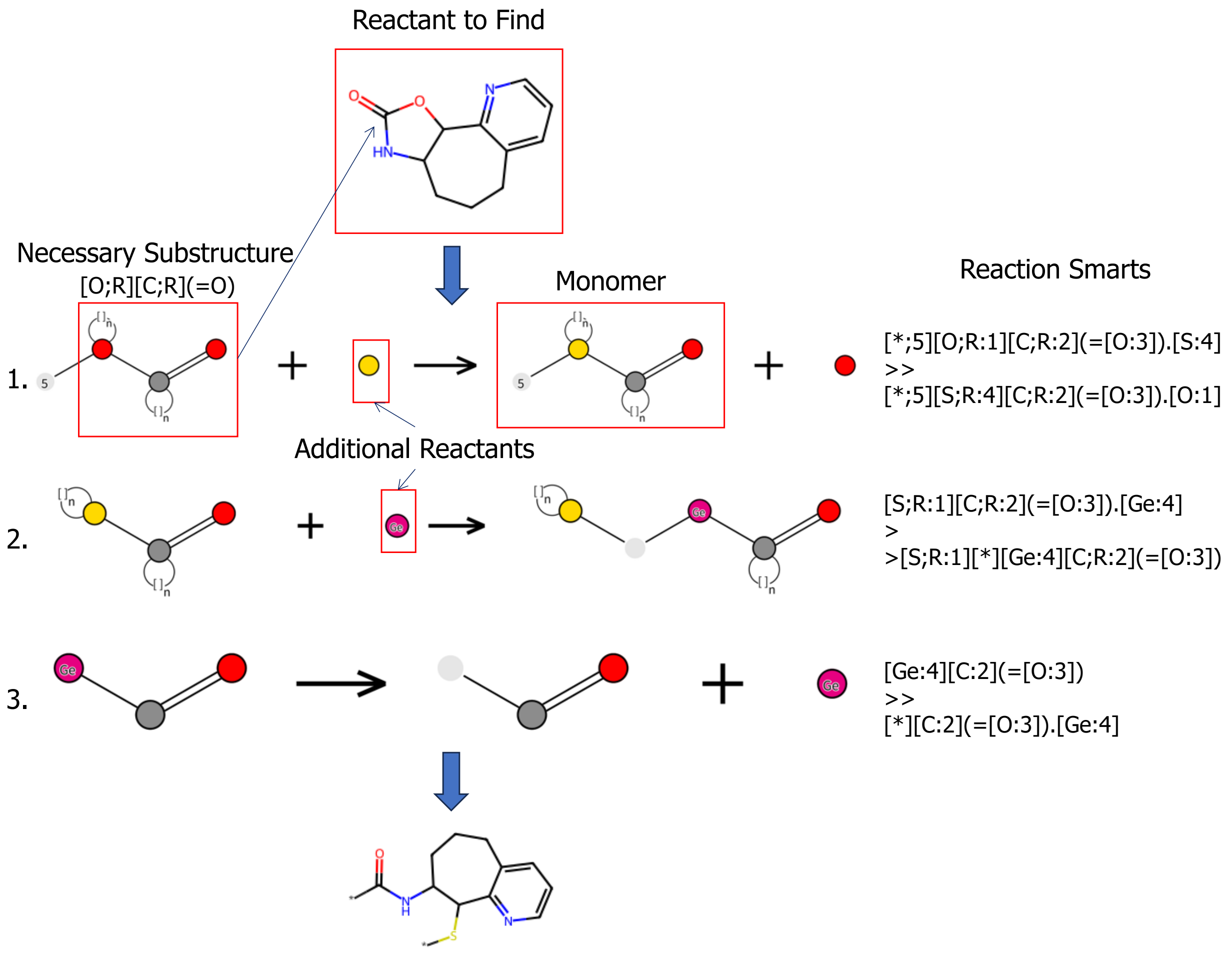


Figure S6: Illustration of VFS Procedure. In this example, an ester is being converted to a thioester, then having its ring opened in three steps. The first steps see the non-carbonyl oxygen replaced with a sulfur. Following that the ring-opening process occurs in two steps. First, a germanium atom and star are embedded between the sulfur and carbonyl group so the star can be added to the final SMILES. Germanium was chosen as it is rare to find in polymer materials and is used to break the ring through reaction SMILES arbitrary target specification (SMARTS). The final step involves removing the germanium and replacing it with a star, which acts to open the ring of the monomer and create a valid polymer structure. Reaction figures generated via SMARTSviewer.[3]

possible to designate a particular step as the monomer generating step. In this scenario, the output from this step can be retained and stored as a hypothetical molecule within the molecules table. This step becomes crucial when molecules need to undergo transformation into monomers before proceeding to polymerization. This is especially pertinent for ring-opening polymerization (ROP) polymers because the enthalpy of polymerization ($\Delta H$) is calculated from the structure of the monomer and polymer. In Figure S6 this would occur after step 1.

The variable reactants defined in the reactant to find table, which catalogs their association with a specific reaction procedure, the designated step for their inclusion, and links to the necessary and unacceptable substructures tables, which track the substructures to be contained or avoided. In cases where a certain number of instances of a particular molecule substructure are required, such specifications are documented within this framework. For example, in Figure S6, the requirement for only one ester within a ring is stipulated to govern the type of ROP reaction that transpires.

When a user passes in their reaction procedure, the necessary and unacceptable substructure SMARTS for each variable reactant are initially stored within the substructure table and subsequently linked to the molecules table through a dedicated molecule substructures table. This normalized table setup enables us to query molecules with specific substructures via the the indexed substructure ID, which improves query performance. We order molecules by their ID and search for the substructures in batches using RDKit in our codebase, keeping track of if the substructure appears and how often.[4] We retain a record of the last searched molecule in order to speed up searches in scenarios where new molecules are introduced to the database or if the search process is temporarily halted. In Figure S6, this search would be for the ester structure contained within a ring according to the SMARTS query in the box.

After cataloging all requisite substructures, we proceed to extract molecules that encompass the necessary substructures in the correct quantity while excluding any contain-

ing unacceptable substructures. This process is carried out through a SQL query, filtering out molecules with SAScore scores exceeding seven. To manage memory efficiently, these molecules are sorted by their unique molecule IDs and processed in batches. The offsets for these batches are recorded in the database, allowing us to restart the reaction procedure at the last set of molecules processed if additional molecules are introduced to the database. Furthermore, to expedite the generation of polymers and fingerprints, we harness multiple CPU cores, optimizing the overall efficiency of the operation.

As the molecules run through the reaction, the polymers output at the end of the last reaction step have their SMILES canonicalized. This canonical SMILES is then used to query the homopolymers table in the database, which benefits from a B-Tree index specifically created on the canonical SMILES. If the polymer already exists within the database, its unique polymer ID is retrieved. However, if the polymer is not yet cataloged, its SMILES, canonical SMILES, and categorization (hypothetical) are stored in the homopolymers table.

Upon saving, each homopolymer is automatically assigned a distinct polymer ID within the polymers table, as illustrated on the right-hand side of Figure S5. This polymers table serves as a central mapping that links between the homopolymers and copolymers table, although the exploration of copolymers is beyond the scope of this study.

The polymer ID, monomer ID (if a monomer generation step was defined) and reaction procedure ID are stored in the reaction polymer mappings table and a unique ID is created. This ID is linked to the molecules used in the reaction and the step at which each molecule was used via the reaction found reactant map in the center of Figure S5. This capability enables us to conveniently trace the origin of specific polymers, along with the corresponding reaction procedures and the reactants utilized in their creation.

Furthermore, alongside the tables pertaining to the VFS process, we also maintain additional tables that encompass experimentally measured or computationally simulated (DFT, MD) properties of polymers, as depicted on the rightmost side of Figure S5. Additionally, we house tables containing machine learning predicted properties of polymers, positioned

on the lower right side of Figure S5. These properties serve as invaluable resources for the development of machine learning models and aid in the conception of hypothetical polymer designs.

By structuring our database in this manner, the extraction of candidate polymers becomes a seamless process facilitated by straightforward SQL queries.

## Reaction Procedures

The supplementary file "reaction_procedures.json" (found in our polyVERSE repository on GitHub) presents a comprehensive inventory of reaction procedures in a structured JavaScript object notation (JSON) format. Each entry encapsulates the class of the monomer being manipulated alongside the corresponding reaction procedures. These procedures comprise a sequence of reactions, with each step delineated by its reaction SMARTS and a succinct description of its intended outcome. Additionally, the requisite reactant SMILES are delineated, along with specifications regarding which reactants must be queried from the database. These reactants are characterized by lists of essential and prohibited substructures, each defined by their respective SMARTS notation. The presence of necessary substructures within the reactants is restricted to be between a minimum and maximum value, while no such restriction is provided for unacceptable substructures. For a reactant to be deemed suitable, it must possess all requisite substructures within in the provided range while excluding any flagged as unacceptable.

## Webscraper

We developed a specialized web scraper (available on GitHub) for acquiring molecular data from VWR, a prominent supplier for research laboratories, and its collaborator eMolecules.[5,6] The eMolecules platform enables three distinct search modalities: exact structure, substructure, and similarity-based searches. Users can input molecular structures either directly or

by uploading a .mol file. Search results are typically displayed in a tabular format, with extensive listings sometimes exceeding 45,000 molecules in over 9,000 pages.

Each molecule listing includes a button for accessing detailed information, such as source, Chemical Abstracts Service (CAS) number, SMILES notation, names, supplier-specific IDs, molecular weight, and formula. A "more info" button leads to a table with supplier-specific pricing and quantity options.

Given the enormity of the data involved, especially for complex searches like terminal alkynes, manual data extraction is impractical. To address this, we employed a systematic web scraping process outlined below:

Below is a step-by-step process of how the scraper works:

1. **User Input**: A list of target substructures, provided in SMILES notation.

2. **SMILES to .mol Conversion**: Conversion of SMILES strings to .mol format using the RDKit cheminformatics toolkit.[4]

3. **Website Navigation Setup**: Utilization of Selenium for automating navigation to VWR's molecule search and subsequent login to eMolecules.[6,7]

4. **Initial Setup**: The scraper clears any previous queries and prepares for a new search by selecting the "Import Molfile" option and pasting the substructure (in .mol file format) into the prompt opened.

5. **Initiate Substructure Search**: The scraper clicks on the "Import" button to load the substructure data and then the "Substructure Search" button to begin searching for compounds matching the provided substructure.

6. **Data Extraction Loop**: For each compound found:

    (a) Detailed information is accessed, and data such as names, properties, and IDs are extracted using BeautifulSoup.[8]

(b) Price information is retrieved by clicking ”more info” and extracting supplier, amount, unit, and price details.

(c) All data is compiled into a JSON file.

7. **Navigate to Next Table**: The scraper navigates to the next table of search results to repeat the data extraction process for the next set of compounds.

8. **Repeat or Exit**: Once all tables have been searched or terms and condition limits have been met for the day, the scraper navigates to the eMolecules site and initiates the next substructure query if there are more substructures to search for. If there are no more substructures left to search, the process exits.

This approach enables the retrieval of highly accurate pricing information for molecules, distinguishing itself from our other databases like the eMolecules database dump, Zinc15, and ChemBL. It adds an extra dimension to our screening process for potential polymers. However, we proceeded cautiously to ensure compliance with the terms of service for these searches, resulting in a slower extraction process. As a consequence, we can feasibly extract only a few thousand data points over the course of a few days. Although comprehensive pricing datasets are accessible for purchase from eMolecules, procuring them was not viable given the financial constraints of our current project.

Leveraging our web scraping tool, we successfully extracted data on 45,842 molecules featuring terminal alkynes, used for the hypothetical thiocane reactions. Our analysis revealed that 329 of these molecules were not available for purchase within the U.S., and 3,380 lacked pricing information. For the remaining 42,462 molecules, we gathered a comprehensive dataset of 315,526 price points, offered by various vendors and spanning different concentrations. For instance, the molecule C#CC#N was available in multiple forms, such as 1 gram from BetaPharma at 770 USD, 5 grams for 844 USD, or 100 mg for 844.00 USD from Syngene International.

The next step involved processing the molecule SMILES and associated price data for

integration into our relational database. Utilizing RDKit, we canonicalized the SMILES strings, ensuring database queries first checked for existing entries to avoid duplicates. If a molecule was already cataloged, we retrieved its unique identifier; if not, it was inserted into the database, followed by the retrieval of its ID for linkage to our price information.

# References


(1) Kuenneth, C.; Rajan, A. C.; Tran, H.; Chen, L.; Kim, C.; Ramprasad, R. Polymer Informatics with Multi-Task Learning. *Patterns* **2021**, *2*, 100238.

(2) Oh, K.; Kim, H.; Cardelli, F.; Bwititi, T.; Martynow, A. M. Synthesis of Cyclic Thioethers through Tandem C(sp3)-S and C(sp2)-S Bond Formations from alpha,beta'-Dichloro Vinyl Ketones. *The Journal of Organic Chemistry* **2008**, *73*, 2432–2434.

(3) ZBH, C. f. B. H. SMARTS.Plus. https://smarts.plus/smartsview.

(4) RDKit. https://www.rdkit.org/.

(5) VWR, Part of Avantor - Chemicals and Laboratory Scientific Supplies. https://us.vwr.com/store/.

(6) Vwr.eMolecules.Com | Chemical Structure Drawing Search - eMolecules. https://vwr.emolecules.com/index.php.

(7) Chemical Structure Search | VWR. https://us.vwr.com/store/search/searchMol.jsp.

(8) Beautiful Soup Documentation — Beautiful Soup 4.12.0 Documentation. https://www.crummy.com/software/BeautifulSoup/bs4/doc/.

# Glossary

$T_g$ glass transition temperature. 1–3

$T_m$ melting temperature. 1–3

$\Delta H$ enthalpy of polymerization. 10

$\sigma_b$ tensile strength at break. 1–3

**CAS** Chemical Abstracts Service. 13

**E** Young's modulus. 1–3

**JSON** JavaScript object notation. 12

**ROP** ring-opening polymerization. 10

**SAScore** synthetic accessibility score. 7, 11

**SMARTS** SMILES arbitrary target specification. 8–10, 12

**SMILES** simplified molecular-input line-entry system. 7, 9, 11–15

**SQL** structured query language. 6, 11, 12

**VFS** virtual forward synthesis. 6–9, 11
